# Supplementary material for: Tuning effective hyperfine fields in PEDOT:PSS thin films by doping
Source: arXiv:1804.05139 ancillary file (2018-04-14)
Supplement: Supplementary file 1 [file supplemental.pdf]

# Supplemental Materials: Tuning effective hyperfine fields in PEDOT:PSS thin films by doping

M. Y. Teferi,[1] J. Ogle,[2] G. Joshi,[1] H. Malissa,[1] S. Jamali,[1] D. L. Baird,[1] J. M. Lupton,[3] L. Whittaker Brooks,[2] and C. Boehme[1]

[1]*Department of Physics and Astronomy, University of Utah, Salt Lake City, Utah 84112, USA*

[2]*Department of Chemistry, University of Utah, Salt Lake City, Utah 84112, USA*

[3]*Institut für Experimetalle und Angewandte Physik, Universität Regensburg, Resensburg, Germany*

## DETERMINATION OF CHARGE CARRIER MOBILITIES AT LOW TEMPERATURES

The room temperature current-voltage (IV) characteristics of the (PEDOT:PSS) devices used in this study revealed that all samples were all highly conductive with purely Ohmic behavior and the resistance gradually decreasing with increasing EG doping density, as shown in Fig. S1(a)], as expected from previous studies [S1, S2]. We note that the relative device resistance changes measured here deviate strongly from literature reports as they contain series resistance contributions due to the thin-film wiring of the EDMR templates.

At $T = 5\,\text{K}$, higher EG density also leads to higher currents, however, no Ohmic behavior is seen as the IV characterstics becomes highly non-linear as shown in Fig. 2(a) of the article. Schottky barriers at the interfaces between the PEDOT:PSS layer and the two contact materials can be excluded as the origin of these non-linearities since all IV curves show symmetric behavior, even though the two contact materials (ITO and Al) have different work functions. We note that the Ohmic nature of the two contacts ITO/PEDOT:PSS and PEDOT:PSS/Al is well established [S3]. Therefore, the non-linearity of the IV characteristics can be attribute to space-charge limited conduction, implying that charge transport occurs due to random transitions between localized states (traps). In this case, distinct bias-dependent transport regimes exist: at low bias the current density is given by $J = qp\mu V/d$ with $q$ being the elementary charge, $p$ the charge carrier density, $\mu$ the carrier mobility, $V$

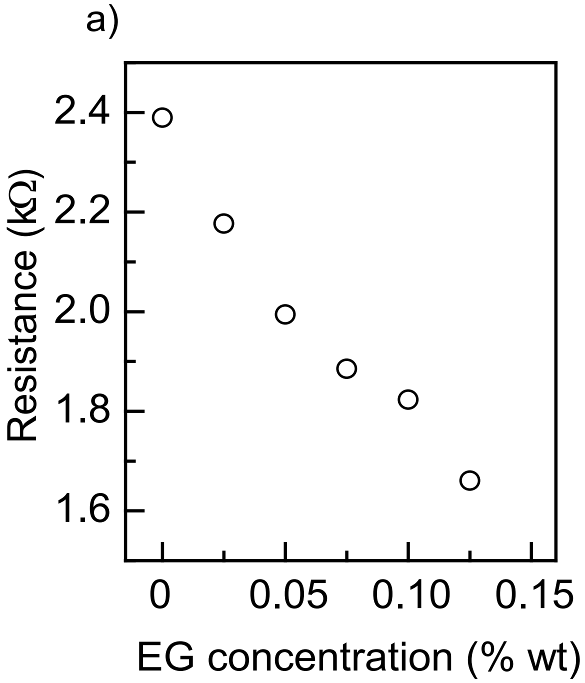


FIG. S1. (a) Electrical characterization of the PEDOT:PSS thin-film devices for different EG doping concentrations at room temperature. The plot represents the device resistances as a function of the EG doping concentrations. The IV measurements used to obtain these values (not shown here) were linear (Ohmic) within the noise levels. (b) Log-log plot of the low-temperature IV data for 0.05% EG doping as shown in Fig. 1(a) of the main text as well as fits of a linear and a quadratic function to the data within the low-bias and high-bias regimes. Within the indicated ranges 1 and 3, the measured data shows good agreement with the fit functions. Between these two regions, a more complex behavior is seen.

the applied voltage, and d the film thickness [S4, S5]. Above the bias where the distribution of occupied trap states becomes significant, $J \propto V^{l+1}/d^{2l+1}$ follows a power-law dependence, with $l$ being an energy parameter. Beyond a second bias threshold when trap-filled space charges exist,

$$J = \frac{9}{8}\epsilon_0\epsilon_r\mu_{\text{eff}}\frac{V^2}{d^3}$$

will be described by the Mott-Gurney square law, where $\epsilon_r$ is the relative dielectric constant of the film, $\epsilon_0$ is the free-space permittivity and $\mu_{\text{eff}}$ is the effective charge carrier mobility

for holes and electrons given by

$$\mu_{\text{eff}} = \frac{2}{3}\sqrt{2\pi\frac{\mu_e\mu_h}{\mu_r}\left(\mu_e+\mu_h\right)} \quad .$$

Figure S1(b) displays a double-logarithmic plot of the data in Fig. 2(a) for 0.05% EG doped PEDOT:PSS and two fits with linear and quadratic bias dependencies, applied to the data within the low-bias and high-bias regimes, respectively. These fits confirm good agreement with the data, and therefore, the conduction is attributed to space charge limited transport. The fits then allow for the determination of $\mu_{\text{eff}}$ assuming $\epsilon_r \approx 2.2$ and a profilometer measured film thickness of ∼50 nm.

Figure 2(b) displays the results of a repetition of this procedure for all EG doping concentrations studied. While these mobilities are determined from low temperature IV curves and are several orders of magnitude smaller than the room-temperature mobilities they still confirm previous observations of mobility increase in PEDOT:PSS films with increasing EG concentrations [S6] which have been attributed to EG induced structural reorganization (i.e. changes to the film morphology) and conformational changes of the PEDOT polymer from a coiled to an extended (linear) structure [S6–S8]. This result shows that for the samples used in this study, good control of $\mu_{\text{eff}}$ through EG doping is achieved, allowing for a study of effective hyperfine field strengths and spin-coherence times within these devices as a function of mobility that is presented in the article.

---


[S1] J. Nevrela et al., *J. Polym. Sci. Part B: Polym. Phys.* **53**, 1139 (2015).

[S2] A. M. Nardes et al., *Adv. Mater.* **19**, 1196 (2007).

[S3] S. A. Rutledge and A. S. Helmey, *J. Appl. Phys.* **114**, 133708 (2013).

[S4] M. A. Lampert, *Phys. Rev.* **103**, 1648 (1956).

[S5] M. A. Lampert and P. Mark, *Current Injection in Solids.* Academic press, New York, 1970.

[S6] Q. Wei, M. Masakazu, Y. Naitoh, and T. Ishida, *Adv. Mater.* **25**, 2831 (2013).

[S7] H. Shi, C. Liu, Q. Jiang, and J. K. Xu, *Adv. Electron. Mater.* **1**, 150017 (2015).

[S8] J. Ouyang, C.-W. Chu, F.-Chen, and Q. X. Y. Yang, *Adv. Funct. Mater.* **15**, 203 (2005).
